# Supplementary material for: High-frequency asymptotic behavior of self-energies in quantum impurity models
Source: arXiv:1107.5536 source file (2011-07-27)
Supplement: Supplementary file 1 [file Asymptotics_supplementary.pdf]

# Program to calculate high frequency asymptotics of self-energies for n-orbital model with rotationally invariant Slater-Kanamori Interaction

X. Wang, H. T. Dang, and A. J. Millis
June-July 2011

## Initialize

Download sneg library from http://nrgljubljana.ijs.si/sneg/sneg.m and place in the working directory.

Set mathematica directory to the working directory which contains sneg.m

```
SetDirectory["/your/working/directory"];
```

Load sneg library

```
In[1]:= << sneg`
```

```
sneg 1.228 Copyright (C) 2011 Rok Zitko
```

```
Out[1]= sneg.m $Id: sneg.m,v 1.228 2011/03/17 13:14:24 rokzitko Exp rokzitko $ loaded
```

Set recursion and iteration limits according to size of problem

```
In[2]:= $RecursionLimit = 2000;
        $IterationLimit = 8000;
```

Define fermion operators for sneg calculation (d: impurity model operator)

```
In[4]:= snegfermionoperators[d];
```

Define non-Hubbard interactions (exchange and pairing interactions)

```
In[5]:= exchange[op1_?fermionQ[j1___], op2_?fermionQ[j2___]] :=
          nc[op1[CR, j1, DO], op2[CR, j2, UP], op2[AN, j2, DO], op1[AN, j1, UP]] +
           nc[op1[CR, j1, UP], op2[CR, j2, DO], op2[AN, j2, UP], op1[AN, j1, DO]];
        pairing[op1_?fermionQ[j1___], op2_?fermionQ[j2___]] :=
          nc[op1[CR, j1, DO], op1[CR, j1, UP], op2[AN, j2, DO], op2[AN, j2, UP]] +
           nc[op2[CR, j2, DO], op2[CR, j2, UP], op1[AN, j1, DO], op1[AN, j1, UP]];
```

Define interaction constants

```
In[7]:= snegrealconstants[U];
        snegrealconstants[U1];
        snegrealconstants[J];
```

## Do calculation

At high frequencies the self energy is

$\Sigma = \Sigma_\infty + \Sigma_1/i\omega_n$

The coefficients are given by

$\Sigma_\infty = -\langle\{[H, d], d^+\}\rangle$,
$\Sigma_1 = \langle\{[H, [H, d]], d^+\}\rangle - (\Sigma_\infty)^2$.

In the following *Mathematica* code, we calculate all the commutators and anticommutators. To get the high frequency coefficients, one only needs to take the average of these results. In our calculations, the notations are

res1 = $[H, d_{\alpha\sigma}]$,
res2 = $[H, [H, d_{\alpha\sigma}]]$,
$\Sigma_\infty = -\{[H, d], d^+\}$,
$G_2 = \{[H, [H, d]], d^+\}$.

In the following, we demonstrate the code for 5-band, 1-band, 2-band, and 3-band models.

### Example : 5-band model

We use the 5-band Slater-Kanamori model as an example.
Set number of orbitals nOrb (nOrb=5 in this example) and define the Hamiltonian.
The Hamiltonian is set to be the interacting one, the kinetic part of the Hamiltonian is excluded in this calculation.

```
nOrb = 5;
Hint = U Sum[hubbard[d[n]], {n, nOrb}] +
    (U1 - J) Sum[number[d[n], UP] ~nc~ number[d[m], UP], {n, nOrb}, {m, n + 1, nOrb}] +
    (U1 - J) Sum[number[d[n], DO] ~nc~ number[d[m], DO], {n, nOrb}, {m, n + 1, nOrb}] +
    U1 ~nc~ Sum[If[n ≠ m, number[d[n], UP] ~nc~ number[d[m], DO], 0], {n, nOrb}, {m, nOrb}] -
    J (Sum[exchange[d[n], d[m]] + pairing[d[n], d[m]], {n, nOrb}, {m, n + 1, nOrb}]);
H =
  Hint;
```

Compute $[H, d_{\alpha\sigma}]$

```
res1 = sumFullSimplify[komutator[H, d[AN, 1, UP]]]
```

$-U\, d^\dagger_{1\downarrow}\cdot d_{1\downarrow}\cdot d_{1\Uparrow} - J\, d^\dagger_{1\downarrow}\cdot d_{2\downarrow}\cdot d_{2\Uparrow} - J\, d^\dagger_{1\downarrow}\cdot d_{3\downarrow}\cdot d_{3\Uparrow} - J\, d^\dagger_{1\downarrow}\cdot d_{4\downarrow}\cdot d_{4\Uparrow} - J\, d^\dagger_{1\downarrow}\cdot d_{5\downarrow}\cdot d_{5\Uparrow} - J\, d^\dagger_{2\downarrow}\cdot d_{1\downarrow}\cdot d_{2\Uparrow} + U1\, d^\dagger_{2\downarrow}\cdot d_{1\Uparrow}\cdot d_{2\downarrow} - J\, d^\dagger_{2\Uparrow}\cdot d_{1\Uparrow}\cdot d_{2\Uparrow} + U1\, d^\dagger_{2\Uparrow}\cdot d_{1\Uparrow}\cdot d_{2\Uparrow} - J\, d^\dagger_{3\downarrow}\cdot d_{1\downarrow}\cdot d_{3\Uparrow} + U1\, d^\dagger_{3\downarrow}\cdot d_{1\Uparrow}\cdot d_{3\downarrow} - J\, d^\dagger_{3\Uparrow}\cdot d_{1\Uparrow}\cdot d_{3\Uparrow} + U1\, d^\dagger_{3\Uparrow}\cdot d_{1\Uparrow}\cdot d_{3\Uparrow} - J\, d^\dagger_{4\downarrow}\cdot d_{1\downarrow}\cdot d_{4\Uparrow} + U1\, d^\dagger_{4\downarrow}\cdot d_{1\Uparrow}\cdot d_{4\downarrow} - J\, d^\dagger_{4\Uparrow}\cdot d_{1\Uparrow}\cdot d_{4\Uparrow} + U1\, d^\dagger_{4\Uparrow}\cdot d_{1\Uparrow}\cdot d_{4\Uparrow} - J\, d^\dagger_{5\downarrow}\cdot d_{1\downarrow}\cdot d_{5\Uparrow} + U1\, d^\dagger_{5\downarrow}\cdot d_{1\Uparrow}\cdot d_{5\downarrow} + (-J + U1)\, d^\dagger_{5\Uparrow}\cdot d_{1\Uparrow}\cdot d_{5\Uparrow}$

Compute $[H, [H, d_{\alpha\sigma}]]$ (typically a large output will appear)

```
res2 = komutator[H, res1]
```

A very large output was generated. Here is a sample of it:

$$
\begin{aligned}
&U\Big((-J+U1)\Big(d^\dagger_{1\downarrow}\cdot d^\dagger_{2\downarrow}\cdot d_{1\downarrow}\cdot d_{1\Uparrow}\cdot d_{2\downarrow}+d^\dagger_{1\downarrow}\cdot d^\dagger_{3\downarrow}\cdot d_{1\downarrow}\cdot d_{1\Uparrow}\cdot d_{3\downarrow}+\\
&\quad d^\dagger_{1\downarrow}\cdot d^\dagger_{4\downarrow}\cdot d_{1\downarrow}\cdot d_{1\Uparrow}\cdot d_{4\downarrow}+d^\dagger_{1\downarrow}\cdot d^\dagger_{5\downarrow}\cdot d_{1\downarrow}\cdot d_{1\Uparrow}\cdot d_{5\downarrow}-\\
&\quad d^\dagger_{1\downarrow}\cdot d^\dagger_{2\downarrow}\cdot d^\dagger_{3\downarrow}\cdot d_{1\downarrow}\cdot d_{1\Uparrow}\cdot d_{2\downarrow}\cdot d_{3\downarrow}-d^\dagger_{1\downarrow}\cdot d^\dagger_{2\downarrow}\cdot d^\dagger_{4\downarrow}\cdot d_{1\downarrow}\cdot d_{1\Uparrow}\cdot d_{2\downarrow}\cdot d_{4\downarrow}-\\
&\quad d^\dagger_{1\downarrow}\cdot d^\dagger_{2\downarrow}\cdot d^\dagger_{5\downarrow}\cdot d_{1\downarrow}\cdot d_{1\Uparrow}\cdot d_{2\downarrow}\cdot d_{5\downarrow}-d^\dagger_{1\downarrow}\cdot d^\dagger_{3\downarrow}\cdot d^\dagger_{4\downarrow}\cdot d_{1\downarrow}\cdot d_{1\Uparrow}\cdot d_{3\downarrow}\cdot d_{4\downarrow}-\\
&\quad d^\dagger_{1\downarrow}\cdot d^\dagger_{3\downarrow}\cdot d^\dagger_{5\downarrow}\cdot d_{1\downarrow}\cdot d_{1\Uparrow}\cdot d_{3\downarrow}\cdot d_{5\downarrow}-d^\dagger_{1\downarrow}\cdot d^\dagger_{4\downarrow}\cdot d^\dagger_{5\downarrow}\cdot d_{1\downarrow}\cdot d_{1\Uparrow}\cdot d_{4\downarrow}\cdot d_{5\downarrow}\Big)+\\
&\quad U1\Big(d^\dagger_{1\downarrow}\cdot d^\dagger_{2\downarrow}\cdot d_{1\downarrow}\cdot d_{1\Uparrow}\cdot d_{2\downarrow}+d^\dagger_{1\downarrow}\cdot d^\dagger_{2\Uparrow}\cdot d_{1\downarrow}\cdot d_{1\Uparrow}\cdot d_{2\Uparrow}+\\
&\quad d^\dagger_{1\downarrow}\cdot d^\dagger_{3\downarrow}\cdot d_{1\downarrow}\cdot d_{1\Uparrow}\cdot d_{3\downarrow}+\ll 29\gg\Big)+\\
&\quad (-J+U1)\Big(d^\dagger_{1\downarrow}\cdot d^\dagger_{2\Uparrow}\cdot d_{1\downarrow}\cdot d_{1\Uparrow}\cdot d_{2\Uparrow}+\ll 1\gg+\ll 1\gg+\ll 13\gg\Big)-\\
&\quad J\Big(\ll 44\gg+d^\dagger_{1\downarrow}\cdot d^\dagger_{5\downarrow}\cdot d^\dagger_{5\Uparrow}\cdot d^{\ll 2\gg}_{\ll 1\gg}\cdot d_{\ll 1\gg\ \ll 1\gg}\cdot d_{2\downarrow}\cdot d_{2\Uparrow}+\\
&\quad d^\dagger_{1\downarrow}\cdot d^\dagger_{5\downarrow}\cdot d^\dagger_{5\Uparrow}\cdot d_{1\downarrow}\cdot d_{1\Uparrow}\cdot d_{3\downarrow}\cdot d_{3\Uparrow}+d^\dagger_{1\downarrow}\cdot d^\dagger_{5\downarrow}\cdot d^\dagger_{5\Uparrow}\cdot d_{1\downarrow}\cdot d_{1\Uparrow}\cdot d_{4\downarrow}\cdot d_{4\Uparrow}\Big)+\\
&\quad U\Big(d^\dagger_{1\downarrow}\cdot d_{1\downarrow}\cdot d_{1\Uparrow}-d^\dagger_{1\downarrow}\cdot d^\dagger_{2\downarrow}\cdot d^\dagger_{2\Uparrow}\cdot d_{1\downarrow}\cdot d_{1\Uparrow}\cdot d_{2\downarrow}\cdot d_{2\Uparrow}-\\
&\quad d^\dagger_{1\downarrow}\cdot d^\dagger_{3\downarrow}\cdot d^\dagger_{3\Uparrow}\cdot d_{1\downarrow}\cdot d_{1\Uparrow}\cdot d_{3\downarrow}\cdot d_{3\Uparrow}-d^\dagger_{1\downarrow}\cdot d^\dagger_{4\downarrow}\cdot d^\dagger_{4\Uparrow}\cdot d_{1\downarrow}\cdot d_{1\Uparrow}\cdot d_{4\downarrow}\cdot d_{4\Uparrow}-\\
&\quad d^\dagger_{1\downarrow}\cdot d^\dagger_{5\downarrow}\cdot d^\dagger_{5\Uparrow}\cdot d_{1\downarrow}\cdot d_{1\Uparrow}\cdot d_{5\downarrow}\cdot d_{5\Uparrow}\Big)\Big)+\ll 32\gg+U1\,(\ll 1\gg)
\end{aligned}
$$

Show Less | Show More | Show Full Output | Set Size Limit...

Compute all up-up anticommutator $G_2=\{[H,\ [H,\ d_{\alpha\sigma}]],\ d_{\alpha\sigma}{}^{+}\}$

```
G2 = antikomutator[res2, d[CR, 1, UP]];
sumFullSimplify[G2]
```

$$
\begin{aligned}
&(4J^2+U^2)\,d^\dagger_{1\downarrow}\cdot d_{1\downarrow}+(J^2+U1^2)\,d^\dagger_{2\downarrow}\cdot d_{2\downarrow}+(J-U1)^2\,d^\dagger_{2\Uparrow}\cdot d_{2\Uparrow}+\\
&(J^2+U1^2)\,d^\dagger_{3\downarrow}\cdot d_{3\downarrow}+(J-U1)^2\,d^\dagger_{3\Uparrow}\cdot d_{3\Uparrow}+(J^2+U1^2)\,d^\dagger_{4\downarrow}\cdot d_{4\downarrow}+\\
&J^2\,d^\dagger_{4\Uparrow}\cdot d_{4\Uparrow}-2\,J\,U1\,d^\dagger_{4\Uparrow}\cdot d_{4\Uparrow}+U1^2\,d^\dagger_{4\Uparrow}\cdot d_{4\Uparrow}+J^2\,d^\dagger_{5\downarrow}\cdot d_{5\downarrow}+U1^2\,d^\dagger_{5\downarrow}\cdot d_{5\downarrow}+\\
&J^2\,d^\dagger_{5\Uparrow}\cdot d_{5\Uparrow}-2\,J\,U1\,d^\dagger_{5\Uparrow}\cdot d_{5\Uparrow}+U1^2\,d^\dagger_{5\Uparrow}\cdot d_{5\Uparrow}-2\,J^2\,d^\dagger_{1\downarrow}\cdot d^\dagger_{1\Uparrow}\cdot d_{2\downarrow}\cdot d_{2\Uparrow}-\\
&2\,J\,U\,d^\dagger_{1\downarrow}\cdot d^\dagger_{1\Uparrow}\cdot d_{2\downarrow}\cdot d_{2\Uparrow}+4\,J\,U1\,d^\dagger_{1\downarrow}\cdot d^\dagger_{1\Uparrow}\cdot d_{2\downarrow}\cdot d_{2\Uparrow}-2\,J^2\,d^\dagger_{1\downarrow}\cdot d^\dagger_{1\Uparrow}\cdot d_{3\downarrow}\cdot d_{3\Uparrow}-\\
&2\,J\,U\,d^\dagger_{1\downarrow}\cdot d^\dagger_{1\Uparrow}\cdot d_{3\downarrow}\cdot d_{3\Uparrow}+4\,J\,U1\,d^\dagger_{1\downarrow}\cdot d^\dagger_{1\Uparrow}\cdot d_{3\downarrow}\cdot d_{3\Uparrow}-2\,J^2\,d^\dagger_{1\downarrow}\cdot d^\dagger_{1\Uparrow}\cdot d_{4\downarrow}\cdot d_{4\Uparrow}-\\
&2\,J\,U\,d^\dagger_{1\downarrow}\cdot d^\dagger_{1\Uparrow}\cdot d_{4\downarrow}\cdot d_{4\Uparrow}+4\,J\,U1\,d^\dagger_{1\downarrow}\cdot d^\dagger_{1\Uparrow}\cdot d_{4\downarrow}\cdot d_{4\Uparrow}-2\,J^2\,d^\dagger_{1\downarrow}\cdot d^\dagger_{1\Uparrow}\cdot d_{5\downarrow}\cdot d_{5\Uparrow}-\\
&2\,J\,U\,d^\dagger_{1\downarrow}\cdot d^\dagger_{1\Uparrow}\cdot d_{5\downarrow}\cdot d_{5\Uparrow}+4\,J\,U1\,d^\dagger_{1\downarrow}\cdot d^\dagger_{1\Uparrow}\cdot d_{5\downarrow}\cdot d_{5\Uparrow}+2\,J^2\,d^\dagger_{1\downarrow}\cdot d^\dagger_{2\downarrow}\cdot d_{1\downarrow}\cdot d_{2\downarrow}-
\end{aligned}
$$

$$2\,U\,U1\,d^\dagger_{1\downarrow}\cdot d^\dagger_{2\downarrow}\cdot d_{1\downarrow}\cdot d_{2\downarrow}+2\,J\,U\,d^\dagger_{1\downarrow}\cdot d^\dagger_{2\Uparrow}\cdot d_{1\downarrow}\cdot d_{2\Uparrow}-2\,U\,U1\,d^\dagger_{1\downarrow}\cdot d^\dagger_{2\Uparrow}\cdot d_{1\downarrow}\cdot d_{2\Uparrow}+$$
$$2\,J^2\,d^\dagger_{1\downarrow}\cdot d^\dagger_{3\downarrow}\cdot d_{1\downarrow}\cdot d_{3\downarrow}-2\,U\,U1\,d^\dagger_{1\downarrow}\cdot d^\dagger_{3\downarrow}\cdot d_{1\downarrow}\cdot d_{3\downarrow}+2\,J\,U\,d^\dagger_{1\downarrow}\cdot d^\dagger_{3\Uparrow}\cdot d_{1\downarrow}\cdot d_{3\Uparrow}-$$
$$2\,U\,U1\,d^\dagger_{1\downarrow}\cdot d^\dagger_{3\Uparrow}\cdot d_{1\downarrow}\cdot d_{3\Uparrow}+2\,J^2\,d^\dagger_{1\downarrow}\cdot d^\dagger_{4\downarrow}\cdot d_{1\downarrow}\cdot d_{4\downarrow}-2\,U\,U1\,d^\dagger_{1\downarrow}\cdot d^\dagger_{4\downarrow}\cdot d_{1\downarrow}\cdot d_{4\downarrow}+$$
$$2\,J\,U\,d^\dagger_{1\downarrow}\cdot d^\dagger_{4\Uparrow}\cdot d_{1\downarrow}\cdot d_{4\Uparrow}-2\,U\,U1\,d^\dagger_{1\downarrow}\cdot d^\dagger_{4\Uparrow}\cdot d_{1\downarrow}\cdot d_{4\Uparrow}+2\,J^2\,d^\dagger_{1\downarrow}\cdot d^\dagger_{5\downarrow}\cdot d_{1\downarrow}\cdot d_{5\downarrow}-$$
$$2\,U\,U1\,d^\dagger_{1\downarrow}\cdot d^\dagger_{5\downarrow}\cdot d_{1\downarrow}\cdot d_{5\downarrow}+2\,J\,U\,d^\dagger_{1\downarrow}\cdot d^\dagger_{5\Uparrow}\cdot d_{1\downarrow}\cdot d_{5\Uparrow}-2\,U\,U1\,d^\dagger_{1\downarrow}\cdot d^\dagger_{5\Uparrow}\cdot d_{1\downarrow}\cdot d_{5\Uparrow}+$$
$$2\,J^2\,d^\dagger_{1\Uparrow}\cdot d^\dagger_{2\downarrow}\cdot d_{1\downarrow}\cdot d_{2\Uparrow}-2\,J\,U\,d^\dagger_{1\Uparrow}\cdot d^\dagger_{2\downarrow}\cdot d_{1\downarrow}\cdot d_{2\Uparrow}+2\,J^2\,d^\dagger_{1\Uparrow}\cdot d^\dagger_{3\downarrow}\cdot d_{1\downarrow}\cdot d_{3\Uparrow}-$$
$$2\,J\,U\,d^\dagger_{1\Uparrow}\cdot d^\dagger_{3\downarrow}\cdot d_{1\downarrow}\cdot d_{3\Uparrow}+2\,J^2\,d^\dagger_{1\Uparrow}\cdot d^\dagger_{4\downarrow}\cdot d_{1\downarrow}\cdot d_{4\Uparrow}-2\,J\,U\,d^\dagger_{1\Uparrow}\cdot d^\dagger_{4\downarrow}\cdot d_{1\downarrow}\cdot d_{4\Uparrow}+$$
$$2\,J^2\,d^\dagger_{1\Uparrow}\cdot d^\dagger_{5\downarrow}\cdot d_{1\downarrow}\cdot d_{5\Uparrow}-2\,J\,U\,d^\dagger_{1\Uparrow}\cdot d^\dagger_{5\downarrow}\cdot d_{1\downarrow}\cdot d_{5\Uparrow}+2\,J\,U1\,d^\dagger_{2\downarrow}\cdot d^\dagger_{2\Uparrow}\cdot d_{2\downarrow}\cdot d_{2\Uparrow}-$$
$$2\,U1^2\,d^\dagger_{2\downarrow}\cdot d^\dagger_{2\Uparrow}\cdot d_{2\downarrow}\cdot d_{2\Uparrow}-J^2\,d^\dagger_{2\downarrow}\cdot d^\dagger_{2\Uparrow}\cdot d_{3\downarrow}\cdot d_{3\Uparrow}-J^2\,d^\dagger_{2\downarrow}\cdot d^\dagger_{2\Uparrow}\cdot d_{4\downarrow}\cdot d_{4\Uparrow}-$$
$$J^2\,d^\dagger_{2\downarrow}\cdot d^\dagger_{2\Uparrow}\cdot d_{5\downarrow}\cdot d_{5\Uparrow}-2\,U1^2\,d^\dagger_{2\downarrow}\cdot d^\dagger_{3\downarrow}\cdot d_{2\downarrow}\cdot d_{3\downarrow}+2\,J\,U1\,d^\dagger_{2\downarrow}\cdot d^\dagger_{3\Uparrow}\cdot d_{2\downarrow}\cdot d_{3\Uparrow}-$$
$$2\,U1^2\,d^\dagger_{2\downarrow}\cdot d^\dagger_{3\Uparrow}\cdot d_{2\downarrow}\cdot d_{3\Uparrow}-J^2\,d^\dagger_{2\downarrow}\cdot d^\dagger_{3\Uparrow}\cdot d_{2\Uparrow}\cdot d_{3\downarrow}-2\,U1^2\,d^\dagger_{2\downarrow}\cdot d^\dagger_{4\downarrow}\cdot d_{2\downarrow}\cdot d_{4\downarrow}+$$
$$2\,J\,U1\,d^\dagger_{2\downarrow}\cdot d^\dagger_{4\Uparrow}\cdot d_{2\downarrow}\cdot d_{4\Uparrow}-2\,U1^2\,d^\dagger_{2\downarrow}\cdot d^\dagger_{4\Uparrow}\cdot d_{2\downarrow}\cdot d_{4\Uparrow}-J^2\,d^\dagger_{2\downarrow}\cdot d^\dagger_{4\Uparrow}\cdot d_{2\Uparrow}\cdot d_{4\downarrow}-$$
$$2\,U1^2\,d^\dagger_{2\downarrow}\cdot d^\dagger_{5\downarrow}\cdot d_{2\downarrow}\cdot d_{5\downarrow}+2\,J\,U1\,d^\dagger_{2\downarrow}\cdot d^\dagger_{5\Uparrow}\cdot d_{2\downarrow}\cdot d_{5\Uparrow}-2\,U1^2\,d^\dagger_{2\downarrow}\cdot d^\dagger_{5\Uparrow}\cdot d_{2\downarrow}\cdot d_{5\Uparrow}-$$
$$J^2\,d^\dagger_{2\downarrow}\cdot d^\dagger_{5\Uparrow}\cdot d_{2\Uparrow}\cdot d_{5\downarrow}-J^2\,d^\dagger_{2\Uparrow}\cdot d^\dagger_{3\downarrow}\cdot d_{2\downarrow}\cdot d_{3\Uparrow}+2\,J\,U1\,d^\dagger_{2\Uparrow}\cdot d^\dagger_{3\downarrow}\cdot d_{2\Uparrow}\cdot d_{3\downarrow}-$$
$$2\,U1^2\,d^\dagger_{2\Uparrow}\cdot d^\dagger_{3\downarrow}\cdot d_{2\Uparrow}\cdot d_{3\downarrow}-2\,J^2\,d^\dagger_{2\Uparrow}\cdot d^\dagger_{3\Uparrow}\cdot d_{2\Uparrow}\cdot d_{3\Uparrow}+4\,J\,U1\,d^\dagger_{2\Uparrow}\cdot d^\dagger_{3\Uparrow}\cdot d_{2\Uparrow}\cdot d_{3\Uparrow}-$$
$$2\,U1^2\,d^\dagger_{2\Uparrow}\cdot d^\dagger_{3\Uparrow}\cdot d_{2\Uparrow}\cdot d_{3\Uparrow}-J^2\,d^\dagger_{2\Uparrow}\cdot d^\dagger_{4\downarrow}\cdot d_{2\downarrow}\cdot d_{4\Uparrow}+2\,J\,U1\,d^\dagger_{2\Uparrow}\cdot d^\dagger_{4\downarrow}\cdot d_{2\Uparrow}\cdot d_{4\downarrow}-$$
$$2\,U1^2\,d^\dagger_{2\Uparrow}\cdot d^\dagger_{4\downarrow}\cdot d_{2\Uparrow}\cdot d_{4\downarrow}-2\,J^2\,d^\dagger_{2\Uparrow}\cdot d^\dagger_{4\Uparrow}\cdot d_{2\Uparrow}\cdot d_{4\Uparrow}+4\,J\,U1\,d^\dagger_{2\Uparrow}\cdot d^\dagger_{4\Uparrow}\cdot d_{2\Uparrow}\cdot d_{4\Uparrow}-$$
$$2\,U1^2\,d^\dagger_{2\Uparrow}\cdot d^\dagger_{4\Uparrow}\cdot d_{2\Uparrow}\cdot d_{4\Uparrow}-J^2\,d^\dagger_{2\Uparrow}\cdot d^\dagger_{5\downarrow}\cdot d_{2\downarrow}\cdot d_{5\Uparrow}+2\,J\,U1\,d^\dagger_{2\Uparrow}\cdot d^\dagger_{5\downarrow}\cdot d_{2\Uparrow}\cdot d_{5\downarrow}-$$
$$2\,U1^2\,d^\dagger_{2\Uparrow}\cdot d^\dagger_{5\downarrow}\cdot d_{2\Uparrow}\cdot d_{5\downarrow}-2\,J^2\,d^\dagger_{2\Uparrow}\cdot d^\dagger_{5\Uparrow}\cdot d_{2\Uparrow}\cdot d_{5\Uparrow}+4\,J\,U1\,d^\dagger_{2\Uparrow}\cdot d^\dagger_{5\Uparrow}\cdot d_{2\Uparrow}\cdot d_{5\Uparrow}-$$
$$2\,U1^2\,d^\dagger_{2\Uparrow}\cdot d^\dagger_{5\Uparrow}\cdot d_{2\Uparrow}\cdot d_{5\Uparrow}-J^2\,d^\dagger_{3\downarrow}\cdot d^\dagger_{3\Uparrow}\cdot d_{2\downarrow}\cdot d_{2\Uparrow}+2\,J\,U1\,d^\dagger_{3\downarrow}\cdot d^\dagger_{3\Uparrow}\cdot d_{3\downarrow}\cdot d_{3\Uparrow}-$$
$$2\,U1^2\,d^\dagger_{3\downarrow}\cdot d^\dagger_{3\Uparrow}\cdot d_{3\downarrow}\cdot d_{3\Uparrow}-J^2\,d^\dagger_{3\downarrow}\cdot d^\dagger_{3\Uparrow}\cdot d_{4\downarrow}\cdot d_{4\Uparrow}-J^2\,d^\dagger_{3\downarrow}\cdot d^\dagger_{3\Uparrow}\cdot d_{5\downarrow}\cdot d_{5\Uparrow}-$$
$$2\,U1^2\,d^\dagger_{3\downarrow}\cdot d^\dagger_{4\downarrow}\cdot d_{3\downarrow}\cdot d_{4\downarrow}+2\,J\,U1\,d^\dagger_{3\downarrow}\cdot d^\dagger_{4\Uparrow}\cdot d_{3\downarrow}\cdot d_{4\Uparrow}-2\,U1^2\,d^\dagger_{3\downarrow}\cdot d^\dagger_{4\Uparrow}\cdot d_{3\downarrow}\cdot d_{4\Uparrow}-$$
$$J^2\,d^\dagger_{3\downarrow}\cdot d^\dagger_{4\Uparrow}\cdot d_{3\Uparrow}\cdot d_{4\downarrow}-2\,U1^2\,d^\dagger_{3\downarrow}\cdot d^\dagger_{5\downarrow}\cdot d_{3\downarrow}\cdot d_{5\downarrow}+2\,J\,U1\,d^\dagger_{3\downarrow}\cdot d^\dagger_{5\Uparrow}\cdot d_{3\downarrow}\cdot d_{5\Uparrow}-$$
$$2\,U1^2\,d^\dagger_{3\downarrow}\cdot d^\dagger_{5\Uparrow}\cdot d_{3\downarrow}\cdot d_{5\Uparrow}-J^2\,d^\dagger_{3\downarrow}\cdot d^\dagger_{5\Uparrow}\cdot d_{3\Uparrow}\cdot d_{5\downarrow}-J^2\,d^\dagger_{3\Uparrow}\cdot d^\dagger_{4\downarrow}\cdot d_{3\downarrow}\cdot d_{4\Uparrow}+$$
$$2\,J\,U1\,d^\dagger_{3\Uparrow}\cdot d^\dagger_{4\downarrow}\cdot d_{3\Uparrow}\cdot d_{4\downarrow}-2\,U1^2\,d^\dagger_{3\Uparrow}\cdot d^\dagger_{4\downarrow}\cdot d_{3\Uparrow}\cdot d_{4\downarrow}-2\,J^2\,d^\dagger_{3\Uparrow}\cdot d^\dagger_{4\Uparrow}\cdot d_{3\Uparrow}\cdot d_{4\Uparrow}+$$
$$4\,J\,U1\,d^\dagger_{3\Uparrow}\cdot d^\dagger_{4\Uparrow}\cdot d_{3\Uparrow}\cdot d_{4\Uparrow}-2\,U1^2\,d^\dagger_{3\Uparrow}\cdot d^\dagger_{4\Uparrow}\cdot d_{3\Uparrow}\cdot d_{4\Uparrow}-J^2\,d^\dagger_{3\Uparrow}\cdot d^\dagger_{5\downarrow}\cdot d_{3\downarrow}\cdot d_{5\Uparrow}+$$
$$2\,J\,U1\,d^\dagger_{3\Uparrow}\cdot d^\dagger_{5\downarrow}\cdot d_{3\Uparrow}\cdot d_{5\downarrow}-2\,U1^2\,d^\dagger_{3\Uparrow}\cdot d^\dagger_{5\downarrow}\cdot d_{3\Uparrow}\cdot d_{5\downarrow}-2\,J^2\,d^\dagger_{3\Uparrow}\cdot d^\dagger_{5\Uparrow}\cdot d_{3\Uparrow}\cdot d_{5\Uparrow}+$$
$$4\,J\,U1\,d^\dagger_{3\Uparrow}\cdot d^\dagger_{5\Uparrow}\cdot d_{3\Uparrow}\cdot d_{5\Uparrow}-2\,U1^2\,d^\dagger_{3\Uparrow}\cdot d^\dagger_{5\Uparrow}\cdot d_{3\Uparrow}\cdot d_{5\Uparrow}-J^2\,d^\dagger_{4\downarrow}\cdot d^\dagger_{4\Uparrow}\cdot d_{2\downarrow}\cdot d_{2\Uparrow}-$$
$$J^2\,d^\dagger_{4\downarrow}\cdot d^\dagger_{4\Uparrow}\cdot d_{3\downarrow}\cdot d_{3\Uparrow}+2\,J\,U1\,d^\dagger_{4\downarrow}\cdot d^\dagger_{4\Uparrow}\cdot d_{4\downarrow}\cdot d_{4\Uparrow}-2\,U1^2\,d^\dagger_{4\downarrow}\cdot d^\dagger_{4\Uparrow}\cdot d_{4\downarrow}\cdot d_{4\Uparrow}-$$

$$J^2\, d^\dagger_{4\downarrow}\cdot d^\dagger_{4\Uparrow}\cdot d_{5\downarrow}\cdot d_{5\Uparrow} - 2\,U1^2\, d^\dagger_{4\downarrow}\cdot d^\dagger_{5\downarrow}\cdot d_{4\downarrow}\cdot d_{5\downarrow} + 2\,J\,U1\, d^\dagger_{4\downarrow}\cdot d^\dagger_{5\Uparrow}\cdot d_{4\downarrow}\cdot d_{5\Uparrow} -$$
$$2\,U1^2\, d^\dagger_{4\downarrow}\cdot d^\dagger_{5\Uparrow}\cdot d_{4\downarrow}\cdot d_{5\Uparrow} - J^2\, d^\dagger_{4\downarrow}\cdot d^\dagger_{5\Uparrow}\cdot d_{4\Uparrow}\cdot d_{5\downarrow} - J^2\, d^\dagger_{4\Uparrow}\cdot d^\dagger_{5\downarrow}\cdot d_{4\downarrow}\cdot d_{5\Uparrow} +$$
$$2\,J\,U1\, d^\dagger_{4\Uparrow}\cdot d^\dagger_{5\downarrow}\cdot d_{4\Uparrow}\cdot d_{5\downarrow} - 2\,U1^2\, d^\dagger_{4\Uparrow}\cdot d^\dagger_{5\downarrow}\cdot d_{4\Uparrow}\cdot d_{5\downarrow} - 2\,J^2\, d^\dagger_{4\Uparrow}\cdot d^\dagger_{5\Uparrow}\cdot d_{4\Uparrow}\cdot d_{5\Uparrow} +$$
$$4\,J\,U1\, d^\dagger_{4\Uparrow}\cdot d^\dagger_{5\Uparrow}\cdot d_{4\Uparrow}\cdot d_{5\Uparrow} - 2\,U1^2\, d^\dagger_{4\Uparrow}\cdot d^\dagger_{5\Uparrow}\cdot d_{4\Uparrow}\cdot d_{5\Uparrow} - J^2\, d^\dagger_{5\downarrow}\cdot d^\dagger_{5\Uparrow}\cdot d_{2\downarrow}\cdot d_{2\Uparrow} -$$
$$J^2\, d^\dagger_{5\downarrow}\cdot d^\dagger_{5\Uparrow}\cdot d_{3\downarrow}\cdot d_{3\Uparrow} - J^2\, d^\dagger_{5\downarrow}\cdot d^\dagger_{5\Uparrow}\cdot d_{4\downarrow}\cdot d_{4\Uparrow} + 2\,(J - U1)\,U1\, d^\dagger_{5\downarrow}\cdot d^\dagger_{5\Uparrow}\cdot d_{5\downarrow}\cdot d_{5\Uparrow}$$

Compute up-down anticommutator $\{[H,\ [H,\ d_{\alpha\sigma}]],\ d_{\alpha\bar{\sigma}}{}^{+}\}$

```
G2 ud = antikomutator[res2, d[CR, 1, DO]];
sumFullSimplify[G2 ud]
```

$$-\left(4\,J^2 + U^2\right) d^\dagger_{1\downarrow}\cdot d_{1\Uparrow} - 2\,J\,U1\, d^\dagger_{2\downarrow}\cdot d_{2\Uparrow} - 2\,J\,U1\, d^\dagger_{3\downarrow}\cdot d_{3\Uparrow} -$$
$$2\,J\,U1\, d^\dagger_{4\downarrow}\cdot d_{4\Uparrow} - 2\,J\,U1\, d^\dagger_{5\downarrow}\cdot d_{5\Uparrow} - 2\left(J^2 - U\,U1\right) d^\dagger_{1\downarrow}\cdot d^\dagger_{2\downarrow}\cdot d_{1\Uparrow}\cdot d_{2\downarrow} -$$
$$2\,J\,U\, d^\dagger_{1\downarrow}\cdot d^\dagger_{2\Uparrow}\cdot d_{1\Uparrow}\cdot d_{2\Uparrow} + 2\,U\,U1\, d^\dagger_{1\downarrow}\cdot d^\dagger_{2\Uparrow}\cdot d_{1\Uparrow}\cdot d_{2\Uparrow} - 2\,J^2\, d^\dagger_{1\downarrow}\cdot d^\dagger_{3\downarrow}\cdot d_{1\Uparrow}\cdot d_{3\downarrow} +$$
$$2\,U\,U1\, d^\dagger_{1\downarrow}\cdot d^\dagger_{3\downarrow}\cdot d_{1\Uparrow}\cdot d_{3\downarrow} - 2\,J\,U\, d^\dagger_{1\downarrow}\cdot d^\dagger_{3\Uparrow}\cdot d_{1\Uparrow}\cdot d_{3\Uparrow} + 2\,U\,U1\, d^\dagger_{1\downarrow}\cdot d^\dagger_{3\Uparrow}\cdot d_{1\Uparrow}\cdot d_{3\Uparrow} -$$
$$2\,J^2\, d^\dagger_{1\downarrow}\cdot d^\dagger_{4\downarrow}\cdot d_{1\Uparrow}\cdot d_{4\downarrow} + 2\,U\,U1\, d^\dagger_{1\downarrow}\cdot d^\dagger_{4\downarrow}\cdot d_{1\Uparrow}\cdot d_{4\downarrow} - 2\,J\,U\, d^\dagger_{1\downarrow}\cdot d^\dagger_{4\Uparrow}\cdot d_{1\Uparrow}\cdot d_{4\Uparrow} +$$
$$2\,U\,U1\, d^\dagger_{1\downarrow}\cdot d^\dagger_{4\Uparrow}\cdot d_{1\Uparrow}\cdot d_{4\Uparrow} - 2\,J^2\, d^\dagger_{1\downarrow}\cdot d^\dagger_{5\downarrow}\cdot d_{1\Uparrow}\cdot d_{5\downarrow} + 2\,U\,U1\, d^\dagger_{1\downarrow}\cdot d^\dagger_{5\downarrow}\cdot d_{1\Uparrow}\cdot d_{5\downarrow} -$$
$$2\,J\,U\, d^\dagger_{1\downarrow}\cdot d^\dagger_{5\Uparrow}\cdot d_{1\Uparrow}\cdot d_{5\Uparrow} + 2\,U\,U1\, d^\dagger_{1\downarrow}\cdot d^\dagger_{5\Uparrow}\cdot d_{1\Uparrow}\cdot d_{5\Uparrow} - 2\,J^2\, d^\dagger_{1\Uparrow}\cdot d^\dagger_{2\downarrow}\cdot d_{1\Uparrow}\cdot d_{2\Uparrow} +$$
$$2\,J\,U\, d^\dagger_{1\Uparrow}\cdot d^\dagger_{2\downarrow}\cdot d_{1\Uparrow}\cdot d_{2\Uparrow} - 2\,J^2\, d^\dagger_{1\Uparrow}\cdot d^\dagger_{3\downarrow}\cdot d_{1\Uparrow}\cdot d_{3\Uparrow} + 2\,J\,U\, d^\dagger_{1\Uparrow}\cdot d^\dagger_{3\downarrow}\cdot d_{1\Uparrow}\cdot d_{3\Uparrow} -$$
$$2\,J^2\, d^\dagger_{1\Uparrow}\cdot d^\dagger_{4\downarrow}\cdot d_{1\Uparrow}\cdot d_{4\Uparrow} + 2\,J\,U\, d^\dagger_{1\Uparrow}\cdot d^\dagger_{4\downarrow}\cdot d_{1\Uparrow}\cdot d_{4\Uparrow} - 2\,J^2\, d^\dagger_{1\Uparrow}\cdot d^\dagger_{5\downarrow}\cdot d_{1\Uparrow}\cdot d_{5\Uparrow} +$$
$$2\,J\,U\, d^\dagger_{1\Uparrow}\cdot d^\dagger_{5\downarrow}\cdot d_{1\Uparrow}\cdot d_{5\Uparrow} - J^2\, d^\dagger_{2\downarrow}\cdot d^\dagger_{3\downarrow}\cdot d_{2\downarrow}\cdot d_{3\Uparrow} + 2\,J\,U1\, d^\dagger_{2\downarrow}\cdot d^\dagger_{3\downarrow}\cdot d_{2\downarrow}\cdot d_{3\Uparrow} -$$
$$J^2\, d^\dagger_{2\downarrow}\cdot d^\dagger_{3\downarrow}\cdot d_{2\Uparrow}\cdot d_{3\downarrow} + 2\,J\,U1\, d^\dagger_{2\downarrow}\cdot d^\dagger_{3\downarrow}\cdot d_{2\Uparrow}\cdot d_{3\downarrow} - J^2\, d^\dagger_{2\downarrow}\cdot d^\dagger_{3\Uparrow}\cdot d_{2\Uparrow}\cdot d_{3\Uparrow} +$$
$$2\,J\,U1\, d^\dagger_{2\downarrow}\cdot d^\dagger_{3\Uparrow}\cdot d_{2\Uparrow}\cdot d_{3\Uparrow} - J^2\, d^\dagger_{2\downarrow}\cdot d^\dagger_{4\downarrow}\cdot d_{2\downarrow}\cdot d_{4\Uparrow} + 2\,J\,U1\, d^\dagger_{2\downarrow}\cdot d^\dagger_{4\downarrow}\cdot d_{2\downarrow}\cdot d_{4\Uparrow} -$$
$$J^2\, d^\dagger_{2\downarrow}\cdot d^\dagger_{4\downarrow}\cdot d_{2\Uparrow}\cdot d_{4\downarrow} + 2\,J\,U1\, d^\dagger_{2\downarrow}\cdot d^\dagger_{4\downarrow}\cdot d_{2\Uparrow}\cdot d_{4\downarrow} - J^2\, d^\dagger_{2\downarrow}\cdot d^\dagger_{4\Uparrow}\cdot d_{2\Uparrow}\cdot d_{4\Uparrow} +$$
$$2\,J\,U1\, d^\dagger_{2\downarrow}\cdot d^\dagger_{4\Uparrow}\cdot d_{2\Uparrow}\cdot d_{4\Uparrow} - J^2\, d^\dagger_{2\downarrow}\cdot d^\dagger_{5\downarrow}\cdot d_{2\downarrow}\cdot d_{5\Uparrow} + 2\,J\,U1\, d^\dagger_{2\downarrow}\cdot d^\dagger_{5\downarrow}\cdot d_{2\downarrow}\cdot d_{5\Uparrow} -$$
$$J^2\, d^\dagger_{2\downarrow}\cdot d^\dagger_{5\downarrow}\cdot d_{2\Uparrow}\cdot d_{5\downarrow} + 2\,J\,U1\, d^\dagger_{2\downarrow}\cdot d^\dagger_{5\downarrow}\cdot d_{2\Uparrow}\cdot d_{5\downarrow} - J^2\, d^\dagger_{2\downarrow}\cdot d^\dagger_{5\Uparrow}\cdot d_{2\Uparrow}\cdot d_{5\Uparrow} +$$
$$2\,J\,U1\, d^\dagger_{2\downarrow}\cdot d^\dagger_{5\Uparrow}\cdot d_{2\Uparrow}\cdot d_{5\Uparrow} - J^2\, d^\dagger_{2\Uparrow}\cdot d^\dagger_{3\downarrow}\cdot d_{2\Uparrow}\cdot d_{3\Uparrow} + 2\,J\,U1\, d^\dagger_{2\Uparrow}\cdot d^\dagger_{3\downarrow}\cdot d_{2\Uparrow}\cdot d_{3\Uparrow} -$$
$$J^2\, d^\dagger_{2\Uparrow}\cdot d^\dagger_{4\downarrow}\cdot d_{2\Uparrow}\cdot d_{4\Uparrow} + 2\,J\,U1\, d^\dagger_{2\Uparrow}\cdot d^\dagger_{4\downarrow}\cdot d_{2\Uparrow}\cdot d_{4\Uparrow} - J^2\, d^\dagger_{2\Uparrow}\cdot d^\dagger_{5\downarrow}\cdot d_{2\Uparrow}\cdot d_{5\Uparrow} +$$
$$2\,J\,U1\, d^\dagger_{2\Uparrow}\cdot d^\dagger_{5\downarrow}\cdot d_{2\Uparrow}\cdot d_{5\Uparrow} - J^2\, d^\dagger_{3\downarrow}\cdot d^\dagger_{4\downarrow}\cdot d_{3\downarrow}\cdot d_{4\Uparrow} + 2\,J\,U1\, d^\dagger_{3\downarrow}\cdot d^\dagger_{4\downarrow}\cdot d_{3\downarrow}\cdot d_{4\Uparrow} -$$
$$J^2\, d^\dagger_{3\downarrow}\cdot d^\dagger_{4\downarrow}\cdot d_{3\Uparrow}\cdot d_{4\downarrow} + 2\,J\,U1\, d^\dagger_{3\downarrow}\cdot d^\dagger_{4\downarrow}\cdot d_{3\Uparrow}\cdot d_{4\downarrow} - J^2\, d^\dagger_{3\downarrow}\cdot d^\dagger_{4\Uparrow}\cdot d_{3\Uparrow}\cdot d_{4\Uparrow} +$$
$$2\,J\,U1\, d^\dagger_{3\downarrow}\cdot d^\dagger_{4\Uparrow}\cdot d_{3\Uparrow}\cdot d_{4\Uparrow} - J^2\, d^\dagger_{3\downarrow}\cdot d^\dagger_{5\downarrow}\cdot d_{3\downarrow}\cdot d_{5\Uparrow} + 2\,J\,U1\, d^\dagger_{3\downarrow}\cdot d^\dagger_{5\downarrow}\cdot d_{3\downarrow}\cdot d_{5\Uparrow} -$$
$$J^2\, d^\dagger_{3\downarrow}\cdot d^\dagger_{5\downarrow}\cdot d_{3\Uparrow}\cdot d_{5\downarrow} + 2\,J\,U1\, d^\dagger_{3\downarrow}\cdot d^\dagger_{5\downarrow}\cdot d_{3\Uparrow}\cdot d_{5\downarrow} - J^2\, d^\dagger_{3\downarrow}\cdot d^\dagger_{5\Uparrow}\cdot d_{3\Uparrow}\cdot d_{5\Uparrow} +$$
$$2\,J\,U1\, d^\dagger_{3\downarrow}\cdot d^\dagger_{5\Uparrow}\cdot d_{3\Uparrow}\cdot d_{5\Uparrow} - J^2\, d^\dagger_{3\Uparrow}\cdot d^\dagger_{4\downarrow}\cdot d_{3\Uparrow}\cdot d_{4\Uparrow} + 2\,J\,U1\, d^\dagger_{3\Uparrow}\cdot d^\dagger_{4\downarrow}\cdot d_{3\Uparrow}\cdot d_{4\Uparrow} -$$
$$J^2\, d^\dagger_{3\Uparrow}\cdot d^\dagger_{5\downarrow}\cdot d_{3\Uparrow}\cdot d_{5\Uparrow} + 2\,J\,U1\, d^\dagger_{3\Uparrow}\cdot d^\dagger_{5\downarrow}\cdot d_{3\Uparrow}\cdot d_{5\Uparrow} - J^2\, d^\dagger_{4\downarrow}\cdot d^\dagger_{5\downarrow}\cdot d_{4\downarrow}\cdot d_{5\Uparrow} +$$
$$2\,J\,U1\, d^\dagger_{4\downarrow}\cdot d^\dagger_{5\downarrow}\cdot d_{4\downarrow}\cdot d_{5\Uparrow} - J^2\, d^\dagger_{4\downarrow}\cdot d^\dagger_{5\downarrow}\cdot d_{4\Uparrow}\cdot d_{5\downarrow} + 2\,J\,U1\, d^\dagger_{4\downarrow}\cdot d^\dagger_{5\downarrow}\cdot d_{4\Uparrow}\cdot d_{5\downarrow} -$$
$$J^2\, d^\dagger_{4\downarrow}\cdot d^\dagger_{5\Uparrow}\cdot d_{4\Uparrow}\cdot d_{5\Uparrow} + 2\,J\,U1\, d^\dagger_{4\downarrow}\cdot d^\dagger_{5\Uparrow}\cdot d_{4\Uparrow}\cdot d_{5\Uparrow} - J\,(J - 2\,U1)\, d^\dagger_{4\Uparrow}\cdot d^\dagger_{5\downarrow}\cdot d_{4\Uparrow}\cdot d_{5\Uparrow}$$

Self energy coefficients $\Sigma_\infty$

```
Σ∞ = -antikomutator[res1, d[CR, 1, UP]];
sumFullSimplify[Σ∞]
```

$$U\, d^{\dagger}_{1\downarrow}\cdot d_{1\downarrow} - J\left(d^{\dagger}_{2\Uparrow}\cdot d_{2\Uparrow} + d^{\dagger}_{3\Uparrow}\cdot d_{3\Uparrow} + d^{\dagger}_{4\Uparrow}\cdot d_{4\Uparrow} + d^{\dagger}_{5\Uparrow}\cdot d_{5\Uparrow}\right) + U1\left(d^{\dagger}_{2\downarrow}\cdot d_{2\downarrow} + d^{\dagger}_{2\Uparrow}\cdot d_{2\Uparrow} + d^{\dagger}_{3\downarrow}\cdot d_{3\downarrow} + d^{\dagger}_{3\Uparrow}\cdot d_{3\Uparrow} + d^{\dagger}_{4\downarrow}\cdot d_{4\downarrow} + d^{\dagger}_{4\Uparrow}\cdot d_{4\Uparrow} + d^{\dagger}_{5\downarrow}\cdot d_{5\downarrow} + d^{\dagger}_{5\Uparrow}\cdot d_{5\Uparrow}\right)$$

## Example: 1-band model

In[10]:=
```
nOrb = 1;
Hint = U Sum[hubbard[d[n]], {n, nOrb}] +
    (U1 - J) Sum[number[d[n], UP] ~nc~ number[d[m], UP], {n, nOrb}, {m, n + 1, nOrb}] +
    (U1 - J) Sum[number[d[n], DO] ~nc~ number[d[m], DO], {n, nOrb}, {m, n + 1, nOrb}] +
    U1 ~nc~ Sum[If[n ≠ m, number[d[n], UP] ~nc~ number[d[m], DO], 0], {n, nOrb}, {m, nOrb}] -
    J (Sum[exchange[d[n], d[m]] + pairing[d[n], d[m]], {n, nOrb}, {m, n + 1, nOrb}]);
H = Hint;
res1 = sumFullSimplify[komutator[H, d[AN, 1, UP]]];
res2 = komutator[H, res1];
G2 = antikomutator[res2, d[CR, 1, UP]];
Print["G2=", sumFullSimplify[G2]];
Σ∞ = -antikomutator[res1, d[CR, 1, UP]];
Print["Σ∞=", sumFullSimplify[Σ∞]];
```

$G_2$=$U^2\, d^{\dagger}_{1\downarrow}\cdot d_{1\downarrow}$

$\Sigma_\infty$=$U\, d^{\dagger}_{1\downarrow}\cdot d_{1\downarrow}$

## Example: 2-band model

```
nOrb = 2;
Hint = U Sum[hubbard[d[n]], {n, nOrb}] +
    (U1 - J) Sum[number[d[n], UP] ~nc~ number[d[m], UP], {n, nOrb}, {m, n + 1, nOrb}] +
    (U1 - J) Sum[number[d[n], DO] ~nc~ number[d[m], DO], {n, nOrb}, {m, n + 1, nOrb}] +
    U1 ~nc~ Sum[If[n ≠ m, number[d[n], UP] ~nc~ number[d[m], DO], 0], {n, nOrb}, {m, nOrb}] -
    J (Sum[exchange[d[n], d[m]] + pairing[d[n], d[m]], {n, nOrb}, {m, n + 1, nOrb}]);
H = Hint;
res1 = sumFullSimplify[komutator[H, d[AN, 1, UP]]];
res2 = komutator[H, res1];
G2 = antikomutator[res2, d[CR, 1, UP]];
Print["G2=", sumFullSimplify[G2]];
Σ∞ = -antikomutator[res1, d[CR, 1, UP]];
Print["Σ∞=", sumFullSimplify[Σ∞]];
```

$G_2$=$\left(J^2 + U^2\right) d^{\dagger}_{1\downarrow}\cdot d_{1\downarrow} + \left(J^2 + U1^2\right) d^{\dagger}_{2\downarrow}\cdot d_{2\downarrow} + (J - U1)^2\, d^{\dagger}_{2\Uparrow}\cdot d_{2\Uparrow} - 2\left(J\,(J + U - 2\,U1)\, d^{\dagger}_{1\downarrow}\cdot d^{\dagger}_{1\Uparrow}\cdot d_{2\downarrow}\cdot d_{2\Uparrow} + \left(-J^2 + U\,U1\right) d^{\dagger}_{1\downarrow}\cdot d^{\dagger}_{2\downarrow}\cdot d_{1\downarrow}\cdot d_{2\downarrow} + U\,(-J + U1)\, d^{\dagger}_{1\downarrow}\cdot d^{\dagger}_{2\Uparrow}\cdot d_{1\downarrow}\cdot d_{2\Uparrow} + J\,(-J + U)\, d^{\dagger}_{1\Uparrow}\cdot d^{\dagger}_{2\downarrow}\cdot d_{1\downarrow}\cdot d_{2\Uparrow} + U1\,(-J + U1)\, d^{\dagger}_{2\downarrow}\cdot d^{\dagger}_{2\Uparrow}\cdot d_{2\downarrow}\cdot d_{2\Uparrow}\right)$

$\Sigma_\infty$=$U\, d^{\dagger}_{1\downarrow}\cdot d_{1\downarrow} + U1\, d^{\dagger}_{2\downarrow}\cdot d_{2\downarrow} + (-J + U1)\, d^{\dagger}_{2\Uparrow}\cdot d_{2\Uparrow}$

## Example: 3-band model

```
nOrb = 3;
Hint = U Sum[hubbard[d[n]], {n, nOrb}] +
    (U1 - J) Sum[number[d[n], UP] ~nc~ number[d[m], UP], {n, nOrb}, {m, n + 1, nOrb}] +
    (U1 - J) Sum[number[d[n], DO] ~nc~ number[d[m], DO], {n, nOrb}, {m, n + 1, nOrb}] +
    U1 ~nc~ Sum[If[n ≠ m, number[d[n], UP] ~nc~ number[d[m], DO], 0], {n, nOrb}, {m, nOrb}] -
    J (Sum[exchange[d[n], d[m]] + pairing[d[n], d[m]], {n, nOrb}, {m, n + 1, nOrb}]);
H = Hint;
res1 = sumFullSimplify[komutator[H, d[AN, 1, UP]]];
res2 = komutator[H, res1];
G2 = antikomutator[res2, d[CR, 1, UP]];
Print["G2=", sumFullSimplify[G2]];
Σ∞ = -antikomutator[res1, d[CR, 1, UP]];
Print["Σ∞=", sumFullSimplify[Σ∞]];
```

$$G_2 = \left(2J^2 + U^2\right) d^{\dagger}_{1\downarrow} \cdot d_{1\downarrow} + \left(J^2 + U1^2\right) d^{\dagger}_{2\downarrow} \cdot d_{2\downarrow} + (J - U1)^2 d^{\dagger}_{2\Uparrow} \cdot d_{2\Uparrow} +$$
$$\left(J^2 + U1^2\right) d^{\dagger}_{3\downarrow} \cdot d_{3\downarrow} + (J - U1)^2 d^{\dagger}_{3\Uparrow} \cdot d_{3\Uparrow} - 2J\,(J + U - 2\,U1)\, d^{\dagger}_{1\downarrow} \cdot d^{\dagger}_{1\Uparrow} \cdot d_{2\downarrow} \cdot d_{2\Uparrow} -$$
$$2J^2 d^{\dagger}_{1\downarrow} \cdot d^{\dagger}_{1\Uparrow} \cdot d_{3\downarrow} \cdot d_{3\Uparrow} - 2JU\, d^{\dagger}_{1\downarrow} \cdot d^{\dagger}_{1\Uparrow} \cdot d_{3\downarrow} \cdot d_{3\Uparrow} + 4J\,U1\, d^{\dagger}_{1\downarrow} \cdot d^{\dagger}_{1\Uparrow} \cdot d_{3\downarrow} \cdot d_{3\Uparrow} +$$
$$2J^2 d^{\dagger}_{1\downarrow} \cdot d^{\dagger}_{2\downarrow} \cdot d_{1\downarrow} \cdot d_{2\downarrow} - 2U\,U1\, d^{\dagger}_{1\downarrow} \cdot d^{\dagger}_{2\downarrow} \cdot d_{1\downarrow} \cdot d_{2\downarrow} + 2JU\, d^{\dagger}_{1\downarrow} \cdot d^{\dagger}_{2\Uparrow} \cdot d_{1\downarrow} \cdot d_{2\Uparrow} -$$
$$2U\,U1\, d^{\dagger}_{1\downarrow} \cdot d^{\dagger}_{2\Uparrow} \cdot d_{1\downarrow} \cdot d_{2\Uparrow} + 2J^2 d^{\dagger}_{1\downarrow} \cdot d^{\dagger}_{3\downarrow} \cdot d_{1\downarrow} \cdot d_{3\downarrow} - 2U\,U1\, d^{\dagger}_{1\downarrow} \cdot d^{\dagger}_{3\downarrow} \cdot d_{1\downarrow} \cdot d_{3\downarrow} +$$
$$2JU\, d^{\dagger}_{1\downarrow} \cdot d^{\dagger}_{3\Uparrow} \cdot d_{1\downarrow} \cdot d_{3\Uparrow} - 2U\,U1\, d^{\dagger}_{1\downarrow} \cdot d^{\dagger}_{3\Uparrow} \cdot d_{1\downarrow} \cdot d_{3\Uparrow} + 2J^2 d^{\dagger}_{1\Uparrow} \cdot d^{\dagger}_{2\downarrow} \cdot d_{1\downarrow} \cdot d_{2\Uparrow} -$$
$$2JU\, d^{\dagger}_{1\Uparrow} \cdot d^{\dagger}_{2\downarrow} \cdot d_{1\downarrow} \cdot d_{2\Uparrow} + 2J^2 d^{\dagger}_{1\Uparrow} \cdot d^{\dagger}_{3\downarrow} \cdot d_{1\downarrow} \cdot d_{3\Uparrow} - 2JU\, d^{\dagger}_{1\Uparrow} \cdot d^{\dagger}_{3\downarrow} \cdot d_{1\downarrow} \cdot d_{3\Uparrow} +$$
$$2J\,U1\, d^{\dagger}_{2\downarrow} \cdot d^{\dagger}_{2\Uparrow} \cdot d_{2\downarrow} \cdot d_{2\Uparrow} - 2\,U1^2 d^{\dagger}_{2\downarrow} \cdot d^{\dagger}_{2\Uparrow} \cdot d_{2\downarrow} \cdot d_{2\Uparrow} - J^2 d^{\dagger}_{2\downarrow} \cdot d^{\dagger}_{2\Uparrow} \cdot d_{3\downarrow} \cdot d_{3\Uparrow} -$$
$$2\,U1^2 d^{\dagger}_{2\downarrow} \cdot d^{\dagger}_{3\downarrow} \cdot d_{2\downarrow} \cdot d_{3\downarrow} + 2J\,U1\, d^{\dagger}_{2\downarrow} \cdot d^{\dagger}_{3\Uparrow} \cdot d_{2\downarrow} \cdot d_{3\Uparrow} - 2\,U1^2 d^{\dagger}_{2\downarrow} \cdot d^{\dagger}_{3\Uparrow} \cdot d_{2\downarrow} \cdot d_{3\Uparrow} -$$
$$J^2 d^{\dagger}_{2\downarrow} \cdot d^{\dagger}_{3\Uparrow} \cdot d_{2\Uparrow} \cdot d_{3\downarrow} - J^2 d^{\dagger}_{2\Uparrow} \cdot d^{\dagger}_{3\downarrow} \cdot d_{2\downarrow} \cdot d_{3\Uparrow} + 2J\,U1\, d^{\dagger}_{2\Uparrow} \cdot d^{\dagger}_{3\downarrow} \cdot d_{2\Uparrow} \cdot d_{3\downarrow} -$$
$$2\,U1^2 d^{\dagger}_{2\Uparrow} \cdot d^{\dagger}_{3\downarrow} \cdot d_{2\Uparrow} \cdot d_{3\downarrow} - 2J^2 d^{\dagger}_{2\Uparrow} \cdot d^{\dagger}_{3\Uparrow} \cdot d_{2\Uparrow} \cdot d_{3\Uparrow} + 4J\,U1\, d^{\dagger}_{2\Uparrow} \cdot d^{\dagger}_{3\Uparrow} \cdot d_{2\Uparrow} \cdot d_{3\Uparrow} -$$
$$2\,U1^2 d^{\dagger}_{2\Uparrow} \cdot d^{\dagger}_{3\Uparrow} \cdot d_{2\Uparrow} \cdot d_{3\Uparrow} - J^2 d^{\dagger}_{3\downarrow} \cdot d^{\dagger}_{3\Uparrow} \cdot d_{2\downarrow} \cdot d_{2\Uparrow} + 2\,(J - U1)\,U1\, d^{\dagger}_{3\downarrow} \cdot d^{\dagger}_{3\Uparrow} \cdot d_{3\downarrow} \cdot d_{3\Uparrow}$$

$$\Sigma_\infty = U\, d^{\dagger}_{1\downarrow} \cdot d_{1\downarrow} + U1\, d^{\dagger}_{2\downarrow} \cdot d_{2\downarrow} + (-J + U1)\, d^{\dagger}_{2\Uparrow} \cdot d_{2\Uparrow} + U1\, d^{\dagger}_{3\downarrow} \cdot d_{3\downarrow} + (-J + U1)\, d^{\dagger}_{3\Uparrow} \cdot d_{3\Uparrow}$$
